# Supplementary material for: Efficient event-driven simulations of hard spheres
Source: arXiv:2201.01100 ancillary file (2022-01-04)
Supplement: Supplementary file 1 [file SI.pdf]

# Efficient event-driven simulations of hard spheres – Supplemental Information

Frank Smallenburg
*Université Paris-Saclay, CNRS, Laboratoire de Physique des Solides, 91405 Orsay, France*

### A. Simulation units and output

We simulate systems of $N$ hard spheres in a constant volume $V$ in three dimensions. Each particle $i$ has a position $\mathbf{r}_i$, a diameter $\sigma_i$, a mass $m_i$, and a radius $R_i$. The simulation code operates in the following units:

- Lengths are measured in units of the maximum particle size $\sigma$.
- Mass is measured in units of a reference mass $m$, which is typically chosen to be the mass of a particle with diameter $\sigma$.
- Time is measured in units of $\tau = \sqrt{\beta m \sigma^2}$. Here, $\beta = 1/k_B T$ with $k_B$ Boltzmann's constant.

Note that the simulation assumes that no particles with a diameter greater than $1\sigma$ exist in the simulation, and uses assumption in the creation of the cell list. Hence, all particles necessarily have a diameter $\sigma_i \leq \sigma$. By default, the simulation code sets the mass of all particles to be equal to $m$ when loading an initial configuration, but mass is taken into account when determining the effect of collisions. Hence, other choices for the mass can readily be implemented by adapting the initialization code.

The simulation code measures the pressure $P$ during the simulation, and outputs it in the form of a reduced pressure $P^* = \beta P \sigma^3$. The average pressure in a given time interval $[t_a, t_b]$ is measured via the virial expression

$$P = \rho k_B T + \frac{1}{3V} \frac{\sum \delta \mathbf{p}_i \cdot \mathbf{r}_{ij}}{t_b - t_a}, \quad (1)$$

where $\rho = N/V$ is the number density with $V$ the system volume and $N$ the number of particles, and the sum in the last term is taken over all collisions in the time interval $[t_a, t_b]$. For each collision, $\mathbf{r}_{ij}$ is the center-to-center vector connecting the two colliding particles $i$ and $j$, and $\delta \mathbf{p}_i$ is the momentum change of particle $i$ due to the collision.

Additionally, as a check on conservation of energy, the simulation measures the temperature of the system, using the equipartition theorem

$$\sum_i \frac{1}{2} m v_i^2 = \frac{3N}{2} k_B T. \quad (2)$$

The temperature is reported in units of $m\sigma^2/\tau^2/k_B$, and should be constant during the simulation (up to numerical accuracy). A thermostat function is included in the simulation codes, but is disabled by default. Since the total kinetic energy is a conserved quantity, the temperature remains constant even without a thermostat. Hence, all simulations reported in the main text are performed in the microcanonical ensemble (i.e. at constant total energy).

### B. Compilation and benchmarking details

For the benchmarks presented in the main text, the simulation codes under consideration were compiled using gcc 9.3.0, using optimization flags `-Ofast`, `-funroll-loops`, and `-march=native`. This applies to the **CellList**, **MultiEvent**, and **SingleEvent** codes, as well as the code by Rapaport (Ref. 1). Dynamo [2], version 1.7.6, was compiled from source using the default compilation process outlined in the online documentation.

To emulate CPU loads consistent with normal use in HPC computing, for each benchmark we run multiple identical simulation jobs at the same time, with the number of jobs equal to the number of CPU cores present in the workstation we use for testing. Depending on system size, this leads to a decrease in performance in comparison to running only a single job. As shown in Fig. 1, the impact of running multiple jobs in parallel is strongest at intermediate system sizes ($N \sim 10^4$). We attribute this to the fact that part of the CPU cache is shared between different CPU cores, and hence running only a single simulation results in an effectively larger cache size.

## I. OPTIMIZATION NOTES

### A. Tunable parameters

The EDMD codes presented in the main text each have a small number of optimization parameters that may impact simulation speed.

The most important parameter is the distance over which particles are considered to be nearest neighbors when using a neighbor list. As described in the main text, particles are considered nearest neighbors when their center-to-center distance is smaller than $(1+\alpha)(R_i+R_j)$, where $R_i$ is the radius of particle $i$ and $\alpha$ is the parameter which controls the neighborhood size. Ideally, this shell includes particles in the first shell of neighbors around the central particle, which will be the main candidates for collisions. As shown in Fig. 2, testing with the **SingleEvent** code indicates that $\alpha = 0.5$ is approximately optimal for the higher-density systems, with only a $\sim 10\%$ variation in simulation speed between $\alpha = 0.3$ and 0.7. At lower densities, higher values of

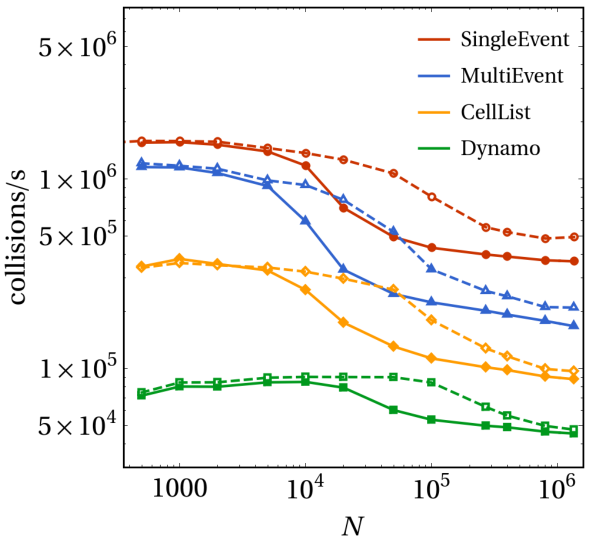


FIG. 1: Comparison between benchmark results performed while running 16 identical simulations in parallel (solid lines) and running only a single job on the benchmarking machine (dashed line).

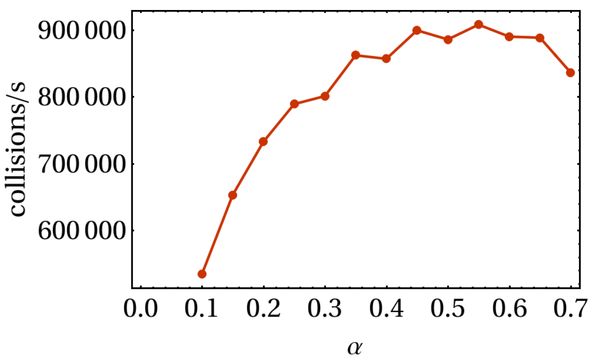


FIG. 2: Performance of the **SingleEvent** code as a function of shell size $\alpha$ for a monodisperse system of $N = 10^4$ particles at packing fraction $\eta = 0.49$. The maximum number of neighbors per particle $n_{\text{neigh}}^{\text{max}}$ was increased to $n_{\text{neigh}}^{\text{max}} = 50$ for the systems with $\alpha \geq 0.6$ test.

$\alpha$ yield slightly better performance, due to the reduced need for neighbor list update events, but the overall impact on simulation speed is minor. In the main text, we use $\alpha = 0.5$ for all systems. Note that the parameter $\alpha$ is incorporated in the simulation as the variable `shellsize` $= 1 + \alpha$

Additionally, the event calendar has a few parameters that may impact performance. In particular, the event calendar structure we use follows Ref. 3, and has two tunable parameters: the length of the time interval $\Delta t$ and the number $n_{\text{lists}}$ of event lists that future events are sorted into. All events within the current time interval of length $\Delta t$ are stored in a binary search tree, while later events are stored in $n_{\text{lists}}$ unsorted linear lists.

Ideally, we choose $\Delta t$ small enough to keep the number of events per time interval small: this ensures a small size of the binary tree, which allows for rapid insertion and deletion of events. Since the typical number of events in any time interval $\Delta t$ is proportional to the number of particles in the system $N$, it is logical to assume that we should choose $\Delta t = cN^{-1}$, with $c$ a constant[3]. In practice, testing for different values of $c$ shows that the exact choice does not significantly impact performance as long as the initial event tree typically contains somewhere between roughly 10 and a few hundred events. In this regime the cost of operating the binary tree is negligible compared to the rest of the simulation code, and further reducing $\Delta t$ does not improve performance. In practice, we use a value of $\Delta t = \tau/N$ for all of our simulations.

Additionally, the event calendar allows for the tuning of the number of event lists $n_{\text{lists}}$. Since events more than $t_{\text{max}} = n_{\text{lists}}\Delta t$ past the start of the current time interval do not fit into any of the $n$lists bins, they are stored in an additional overflow list[3]. Events in the overflow list are rescheduled whenever the last event list is reached, possibly costing significant CPU time if the number of events in the overflow list is large. Hence, ideally the number of events in the overflow list is kept low. In practice, we observe good results for the **SingleEvent** and **MultiEvent** codes using $t_{\text{max}} = \tau$ (i.e. $n$lists $= N$). Based on a Maxwell-Boltzmann distribution of velocities, most particles will experience a neighbor list update event in significantly less time than $\tau$. For the **CellList** code, a significant number of events are scheduled further than $\tau$ into the future, and hence we use $t_{\text{max}} = 5\tau$. However, performance is not strongly dependent on these choices for the cases we investigated.

### B. Nearest image convention

When checking for pair interactions (i.e. for collision predictions, collision handling, or neighbor list updates), we always assume that we are under conditions where the nearest image convention applies[4]. In other words, we only check for interactions of particle $i$ with the periodic image of $j$ that is nearest to particle $i$. This requires that when calculating some interaction between two particles in adjacent cells, they cannot be further apart than half of the box length along any of the Cartesian axes of the simulation box. This can be guaranteed by ensuring that the cell list consists of at least 4 cells along each axis. In practice, this is typically easily satisfied for systems larger than a few hundred particles.

When applying the nearest image convention, the simulation codes makes use of the fact that periodic boundary conditions only need to be considered for particles located in cells at the edge of the simulation box. Hence, each particle carries a flag indicating whether its cell is near an edge, and when calculating a distance between particles $i$ and $j$, periodic boundaries are only considered if this flag is set for particle $i$.

## II. SNAPSHOT FILE FORMAT

The configuration files from the simulation are written in a simple text-based format, which can contain multiple snapshots per file. For each frame, the format consists of $N+2$ lines (with $N$ the number of particles), as follows:

- One line containing just the number of particles
- One line containing the box size, specifying the box length $L_x$, $L_y$, and $L_z$ along the three axes, separated by whitespace.
- One line per particle containing: a letter indicating particle type, three numbers indicating the real-space particle coordinates, and one number indicating the particle radius.

The movie files that are created by the simulation code include multiple of these frames consecutively in a single text file. Note that although the code assumes periodic boundary conditions, coordinates of particles that leave the box during the simulation will be printed as being outside of the simulation box, to allow for analysis of long-time dynamics. Hence, any structural analysis or visualization should apply periodic boundary conditions explicitly.

The simulation codes can read in snapshots in the same format as initial configurations. Periodic boundaries will be applied to the snapshot at the start of the simulation. Note that the simulation code assumes that all box lengths, positions, and radii are given in units of $\sigma$, which is the largest possible particle diameter. Hence, the radius of a particle in the initial configuration should never be given as a number larger than 0.5.

Adaptation to different configuration file formats can be done via modification of the `loadparticles`, `write`, and `outputsnapshot` functions.

## III. CREATING INITIAL CONFIGURATIONS

In addition to the three simulation codes presented in the main text, we include a simulation code where the particles grow in size during the simulation. This allows for a rapid generation of initial configuration files that can then be equilibrated using the other simulation codes.

The **Grow** code used for this is largely identical in setup to the **SingleEvent** code, and is provided along with the simulation codes. It makes use of a thermostat to dissipate excess kinetic energy resulting from collisions between growing particles. System parameters can be adjusted via the global variables at the top of the simulation code. As long as the chosen final packing fraction is not too high, the simulation will output a final snapshot at the desired packing fraction, which can be used as an initial configuration for any of the three simulation codes.

## IV. REFERENCES


[1] D. C. Rapaport and D. C. R. Rapaport, *The art of molecular dynamics simulation* (Cambridge university press, 2004).

[2] M. N. Bannerman, R. Sargant, and L. Lue, Journal of computational chemistry **32**, 3329 (2011).

[3] G. Paul, Journal of Computational Physics **221**, 615 (2007).

[4] D. Frenkel and B. Smit, *Understanding Molecular Simulations: From Algorithms to Applications* (Academic Press, San Diego, 2002).
